# Supplementary material for: Mutual Information of Neural Network Initialisations: Mean Field Approximations
Source: arXiv:2102.04374 source file (2021-02-08)
Supplement: Supplementary file 1 [file appendix.tex]

% \section{Proof of Proposition 1}\label{appendix:gaussian_lb}

% From \cite{hot} we know that 

% \begin{prop}
% Let g(x) be an n-dimensional Gaussian distribution , $\mathcal{N}(\mu, \Lambda)$, with mean $\mu$ and covariance matrix $\Lambda$. If f(x) is an arbitrary distribution with the same mean and covariance matrix, then
% \begin{equation}
%     \mathbb{E}_f[-log(g(x)] = \mathbb{E}_g[-log(g(x)]
% \end{equation}
% \end{prop}
% \begin{proof}
% \begin{align}
%     -\mathbb{E}_f[log(g(X))] & = -\mathbb{E}_f\left[log \frac{1}{\sqrt{(2\pi)^n|\Lambda|}} e^{-\frac{1}{2}(X-\mu)^\top\Lambda^{-1}(X-\mu)}\right] \\
%         &= \frac{1}{2}log (|2\pi\Lambda|) + \frac{log(e)}{2}\mathbb{E}_f\left[ (X-\mu)^\top\Lambda^{-1}(X-\mu)\right]\label{eq:proof_gaussian_var}\\
%         &= \frac{1}{2}log (|2\pi\Lambda|) + \frac{n\log(e)}{2}\label{eq:proof_gaussian_var2}\\
%         &= \frac{1}{2}log (|2\pi e \Lambda|) \label{eq:proof_gaussian_var3}\\
%         &= - \mathbb{E}_g\left[log(g(X)) \right]
% \end{align}
% where in \eqref{eq:proof_gaussian_var} we considered the fact that
% \begin{align}
%     \mathbb{E}\left[(X-\mu)^\top\Lambda^{-1}(X-\mu)\right] & =  \mathbb{E}\left[\sum_{i,j=1}^n(X-\mu)_i^\top(\Lambda^{-1})_{ij}(X-\mu)_j\right] 
%     = \sum_{i,j=1}^n \mathbb{E}\left[(X-\mu)_i^\top(\Lambda^{-1})_{ij}(X-\mu)_j\right] \\
%     &= \sum_{i,j=1}^n (\Lambda^{-1})_{ij}\mathbb{E}\left[(X-\mu)_i^\top(X-\mu)_j\right] = \sum_{i,j=1}^n (\Lambda^{-1})_{ij}\Lambda_{i,j} = \sum_{i,j=1}^n (\Lambda^{-1})_{ij}\Lambda_{j,i} \\
%     &=tr(\Lambda^{-1}\Lambda) = tr(I) = n,
% \end{align}
% and in equation that \eqref{eq:proof_gaussian_var3} since the variable $\textbf{Z}=\Lambda_\textbf{X}^{-1/2}(\textbf{X}- \bm{\mu}) \sim \mathcal{N}(\textbf{0}, \textbf{I})$ with
% \begin{align}
%     \mathbb{E}_\textbf{Z}[-\log(\textbf{Z})] &= - \int_{\mathbb{R}^n} \frac{1}{(2\pi)^{n/2}}e^{-\frac{1}{2}\textbf{y}^\top \textbf{y}}\log\left(\frac{1}{(2\pi)^{n/2}}e^{-\frac{1}{2}\textbf{y}^\top \textbf{y}} \right)d\textbf{y} \\
%     &= \frac{n}{2}\log(2\pi) + \frac{\log(e)}{2}\int_{\mathbb{R}^n} \frac{1}{(2\pi)^{n/2}}e^{-\frac{1}{2}\textbf{y}^\top \textbf{y}}\textbf{y}^\top \textbf{y}d\textbf{y} \\
%     & = \frac{n}{2}\log(2\pi) + \frac{n\log(e)}{2} = \frac{n}{2}\log(2\pi e)
% \end{align}
% the expected logarithm is
% \begin{align}
%     \mathbb{E}_g\left[\log(g) \right]& = \int_{\mathbb{R}^n} g(\textbf{x})\log(g(\textbf{x}))d\textbf{x} \\
%     & = \int_{\mathbb{R}^n} \frac{1}{|\Lambda_\textbf{X}^{-1/2}|} g_\textbf{Z}(\Lambda_\textbf{X}^{-1/2}(\textbf{x}-\bm{\mu})) \log \frac{1}{|\Lambda_\textbf{X}^{-1/2}|} g_\textbf{Z}(\Lambda_\textbf{X}^{-1/2}(\textbf{x}-\bm{\mu}))d\textbf{x}\\
%     &= \int_{\mathbb{R}^n} g_\textbf{Z}(\textbf{z})\log \frac{1}{|\Lambda_\textbf{X}^{-1/2}|}g_\textbf{Z}(\textbf{z})d\textbf{z}\\
%     &= \int_{\mathbb{R}^n} g_\textbf{Z}(\textbf{z})\log g_\textbf{Z}(\textbf{z})d\textbf{z} - \log |\Lambda_\textbf{X}^{-1/2}|\int_{\mathbb{R}^n} g_\textbf{Z}(\textbf{z})d\textbf{z}\\
%     &= \mathbb{E}_\textbf{Z}[\log(\textbf{Z})] - \log|\Lambda_\textbf{X}^{-1/2}|\\
%     &= \frac{n}{2}\log(2\pi e) + \frac{1}{2}\log(|\Lambda_\textbf{X}|) = \frac{1}{2}\log(|2\pi e \Lambda_\textbf{X}|).
% \end{align}

% \end{proof}

% Thus we can show that

% \begin{prop}
% Let g(x,y) be an n-dimensional Gaussian distribution , $\mathcal{N}(\mu, \Lambda)$, with mean $\mu$ an dcovariance matrix $\Lambda$. If f(x,y) is an arbitrary distribution with the same mean and covariance matrix, and with f(x) gaussian, then
% \begin{equation}
%     I_{f_{(xy)}}[X,Y] \geq I_{g_{(xy)}}[X,Y]
% \end{equation}
% \end{prop}
% \begin{proof}
% \begin{align}
%     I_{f}&[X,Y] - I_{g}[X,Y] =  \int_\mathcal{X}\int_\mathcal{Y} f_{\textbf{X},\textbf{Y}}(\textbf{x},\textbf{y})\log \left( \frac{f_{\textbf{X},\textbf{Y}}(\textbf{x},\textbf{y})}{f_{\textbf{X}}(\textbf{x})f_{\textbf{Y}}(\textbf{y})}\right)\ d\textbf{x}\ d\textbf{y} \\
%         & \quad -  \int_\mathcal{X}\int_\mathcal{Y} g_{\textbf{X},\textbf{Y}}(\textbf{x},\textbf{y})\log \left( \frac{g_{\textbf{X},\textbf{Y}}(\textbf{x},\textbf{y})}{g_{\textbf{X}}(\textbf{x})g_{\textbf{Y}}(\textbf{y})}\right)\ d\textbf{x}\ d\textbf{y} \\
%     &= - \int_\mathcal{X} f_\textbf{X}(\textbf{x})\log \left( f_{\textbf{X}}(\textbf{x})\right)\ d\textbf{x} -
%     \int_\mathcal{Y} f_\textbf{Y}(\textbf{y})\log \left( f_{\textbf{Y}}(\textbf{y})\right)\ d\textbf{y} + 
%     \int_\mathcal{X}\int_\mathcal{Y} f_{\textbf{X}\textbf{Y}}(\textbf{x,y})\log \left( f_{\textbf{X}\textbf{Y}}(\textbf{x,y})\right)\ d\textbf{x}d\textbf{y}\\
%         & \quad +\int_\mathcal{X} g_\textbf{X}(\textbf{x})\log \left( g_{\textbf{X}}(\textbf{x})\right)\ d\textbf{x} +
%         \int_\mathcal{Y} g_\textbf{Y}(\textbf{y})\log \left( g_{\textbf{Y}}(\textbf{y})\right)\ d\textbf{y} - 
%         \int_\mathcal{X}\int_\mathcal{Y} g_{\textbf{X}\textbf{Y}}(\textbf{x,y})\log \left( g_{\textbf{X}\textbf{Y}}(\textbf{x,y})\right)\ d\textbf{x}d\textbf{y}\\
%     &= - \int_\mathcal{Y} f_\textbf{Y}(\textbf{y})\log \left( f_{\textbf{Y}}(\textbf{y})\right)\ d\textbf{y} +
%     \int_\mathcal{X}\int_\mathcal{Y} f_{\textbf{X}\textbf{Y}}(\textbf{x,y})\log \left( f_{\textbf{X}\textbf{Y}}(\textbf{x,y})\right)\ d\textbf{x}d\textbf{y}\\
%         & \quad  + \int_\mathcal{Y} g_\textbf{Y}(\textbf{y})\log \left( g_{\textbf{Y}}(\textbf{y})\right)\ d\textbf{y}-
%         \int_\mathcal{X}\int_\mathcal{Y} g_{\textbf{X}\textbf{Y}}(\textbf{x,y})\log \left( g_{\textbf{X}\textbf{Y}}(\textbf{x,y})\right)\ d\textbf{x}d\textbf{y}\\
%     &= \int_\mathcal{Y} f_\textbf{Y}(\textbf{y})\log \left(\frac{g_{\textbf{Y}}(\textbf{y})}{f_{\textbf{Y}}(\textbf{y})} \right)\ d\textbf{y} - 
%         \int_\mathcal{X}\int_\mathcal{Y} f_{\textbf{X}\textbf{Y}}(\textbf{x,y})\log \left( \frac{g_{\textbf{X}\textbf{Y}}(\textbf{x,y})}{f__{\textbf{X}\textbf{Y}}(\textbf{x,y})}\right)\ d\textbf{x}d\textbf{y}\\
%     &= \int_\mathcal{X}\int_\mathcal{Y} f_{\textbf{X}\textbf{Y}}(\textbf{x},\textbf{y})\log \left(\frac{g_{\textbf{Y}}(\textbf{y})}{f_{\textbf{Y}}(\textbf{y})} \right)\ d\textbf{x}d\textbf{y} - 
%         \int_\mathcal{X}\int_\mathcal{Y} f_{\textbf{X}\textbf{Y}}(\textbf{x,y})\log \left( \frac{g_{\textbf{X}\textbf{Y}}(\textbf{x,y})}{f_{\textbf{X}\textbf{Y}}(\textbf{x,y})}\right)\ d\textbf{x}d\textbf{y} \\
%     & = \int_\mathcal{X}\int_\mathcal{Y} f_{\textbf{X}\textbf{Y}}(\textbf{x},\textbf{y})\log \left(\frac{g_{\textbf{Y}}(\textbf{y})}{f_{\textbf{Y}}(\textbf{y})} \frac{f_{\textbf{X}\textbf{Y}}(\textbf{x,y})}{g_{\textbf{X}\textbf{Y}}(\textbf{x,y})}\right)\ d\textbf{x}d\textbf{y}\\
%     & = \int_\mathcal{Y} f_\textbf{Y}(\textbf{y}) \int_\mathcal{X} f_{\textbf{X}|\textbf{Y}}(\textbf{x}|\textbf{Y}=\textbf{y})\log \left( \frac{f_{\textbf{X}|\textbf{Y}}(\textbf{x|Y=y})}{g_{\textbf{X}|\textbf{Y}}(\textbf{x|Y=y})}\right)\ d\textbf{x}d\textbf{y} \\
%     & = \int_\mathcal{Y} f_\textbf{Y}(\textbf{y}) D_{KL}(f_{\textbf{X}|\textbf{Y=y}} || g_{\textbf{X}|\textbf{Y=y}})d\textbf{y} \\
%     & \geq 0
% \end{align}
% where the third equality is due to $f_\textbf{x}$ being gaussian, hence $f_\textbf{x} = g_\textbf{x}$; the fourth is due to Proposition 1
% \end{proof}


% \section{Random Matrix Theory}

% \subsection{Approximation of the Expected log-determinant of \textbf{$\bm{XAX^\top}$}}

% We find an approximation of (I1) and (I2) via a comparison of the covariance matrix $\bm{\Lambda}_{\textbf{h}^{(l)}}$ with a the Wishart matrices $\textbf{X}\sim W_p(\textbf{V},n)$ where the expected log determinant has a close form;
% \begin{equation}
%     \mathbb{E}[\ln|\textbf{X}|] = \varphi_p(\frac{n}{2}) + p \ln(2) + \ln | \textbf{V}|
% \end{equation}
% with $\varphi$ being the digamma function.

% By rewriting the matrix as
% \begin{align}
%     &\Lambda_{\textbf{h}^l} = \mathbb{E}_x[(\textbf{W}^l\sigma(\textbf{h}^l) + \textbf{n}^l + \textbf{b}^l)(\textbf{W}^l\sigma(\textbf{h}^l) + \textbf{n}^l + \textbf{b}^l)^\top]\\
%     &= \left[\textbf{W}^l, \textbf{b}^l + \textbf{n}^l \right] 
%         \begin{bmatrix}
%             \mathbb{E}_\textbf{x}[\sigma(\textbf{h}^l)\sigma(\textbf{h}^l)^\top] & \mathbb{E}_\textbf{x}[\sigma(\textbf{h}^l)] \\
%             \mathbb{E}_\textbf{x}[\sigma(\textbf{h}^l)]^\top &\textbf{I}
%         \end{bmatrix}
%     \left[\textbf{W}^l, \textbf{b}^l + \textbf{n}^l\right]^\top\\
%     &= \textbf{X}
%     \begin{bmatrix}
%         \frac{\sigma_w^2}{n}\mathbb{E}_\textbf{x}[\sigma(\textbf{h}^l)\sigma(\textbf{h}^l)^\top] &\frac{\sqrt{(\sigma_b^2+\sigma_n^2)}\sigma_w}{\sqrt{n}}\mathbb{E}[\sigma(\textbf{h}^l)] \\
%         \frac{\sqrt{(\sigma_b^2+\sigma_n^2)}\sigma_w}{\sqrt{n}}\mathbb{E}[\sigma(\textbf{h}^l)]^\top &(\sigma_b^2+\sigma_n^2)\textbf{I}
%     \end{bmatrix}\textbf{X}^\top \label{eq:matrix_formulation}\\
%     &= \textbf{XAX}^\top
% \end{align}
% where $\textbf{X}\in \mathbb{R}^{n \times n+1}$ and $\textbf{X}_{ij}\sim^{iid}\mathcal{N}(0,1)$, we find a choleski factorisation following \cite{anderson1962introduction} of the product which will allow for an computation of the determinant. 

% \begin{prop}\label{theo:factoriasation}
% Consider a symmetric positive definite matrix $\textbf{A}\in \mathbb{R}^{m\times m}$ and a Gaussian random matrix $\textbf{X} \in \mathbb{R}^{n\times m}$ where the elements are normally distributed. The matrix $\textbf{XAX}^\top$ can be factorised as
% \begin{equation}
%     \textbf{XAX}^\top = \textbf{T}^\top\textbf{T}
% \end{equation}
% where $\textbf{T}$ is an upper diagonal matrix with the diagonal elements being {$\textbf{T}_{ii}\sim \sqrt{\sum_{j=i}^n\lambda_j^{(i)}\chi_1^2} $} where $\lambda_j^{(i)}$ is the j-th eigenvalue of a projection of $\textbf{A}$ to an $n-i+1$ dimensional subspace\footnote{We consider the projection of $A$ to an $n-i+1$ dimensional space generated via $\textbf{O}^\top \textbf{AO}$ with $\textbf{O}\in \mathbb{R}^{n,n-i+1}$ such that $\textbf{O}$^\top$\textbf{O}=\textbf{I}$}.
% \end{prop}
% \begin{proof}
% Since $\textbf{A}$ is spd, it is possible to find an orthonormal matrix such that $\textbf{UAU}^\top = \textbf{D}$ where $D$ is a diagonal matrix whose elements are the eigenvalues of $\textbf{A}$. Further, an orthonormal matrix does not affect the distribution of a Gaussian matrix, i.e. $\textbf{UX}\sim\textbf{X}$, and this allows us to study $\textbf{XDX}^\top$ rather than $\textbf{XAX}^\top$.
% We now define $\tilde{\textbf{X}}$ as 
% \begin{align}
%     &\tilde{\textbf{X}} = 
%     \begin{bmatrix} 
%     &| &| & &|\\
%     &\sqrt{\lambda_1}\textbf{x}_1 &\sqrt{\lambda_2}\textbf{x}_2 & \hdots & \sqrt{\lambda_m}\textbf{x}_{m}\\
%     &| &| & &|
%     \end{bmatrix}
% \end{align}
% and consequently $\textbf{XAX}^\top \sim \tilde{\textbf{X}}\tilde{\textbf{X}}^\top$.

% We now consider a QR factorisation of $\tilde{\textbf{X}}^\top$
% \begin{equation}
%     \tilde{\textbf{X}}^\top = \textbf{O}\textbf{T}
% \end{equation}
% where we can choose the orthogonal matrix following the Grahm-Schmidt algorithm
% \begin{align}
%     \textbf{v}_i &= \left( \tilde{\textbf{X}}_{i,:} - \sum_{j=1}^{i-1}<\tilde{\textbf{X}}_{i,:}, \textbf{o}_j> \textbf{o}_j\right)\\
%     \textbf{o}_i &= \textbf{v}_i / \|\textbf{v}_i \|
% \end{align}
% with $\textbf{v}_1=\tilde{\textbf{X}}_{1,:}$. This implies that $\textbf{T}_{i,j}$ with $j<i$ is the projection of the column $(\tilde{\textbf{X}}^\top)_{:,i}$ over the $j$th column of $\textbf{O}$; i.e.
% \begin{align}
%     \textbf{T}_{ij} =  <\tilde{\textbf{X}}_{i,:}, \textbf{o}_j> \sim \mathcal{N}(0, \sum_k\textbf{O}_{jk}^2\lambda_k).
% \end{align}
% Furthermore, the diagonal elements $ii$ correspond to the norm of vector $\textbf{X} - \sum_{j=1}^{i-1}\textbf{T}_{ij}\textbf{o}_j$ in the space complementary to the one spanned by the vectors $\{\textbf{o}_j\}_{j=1}^{i-1}$. For any basis $\{\hat{\textbf{o}}_j\}_{j=1}^{n-i+1}$  of this complementary space we then obtain that 
% \begin{equation}\label{eq:matr_fact_dist_T}
%     \textbf{T}_{ii}  = \sqrt{\sum_{j=1}^{m-i+1} Y_j^{(i)2}}
% \end{equation}
% where $Y_j^{(i)} = <\tilde{\textbf{X}}_{i,:}, \hat{\textbf{o}}_{j}>$ define the random vector 
% \begin{equation}\label{eq:matr_fact_dist_Y}
%     \textbf{Y}^{(i)}\sim \mathcal{N}\left(\textbf{0},\begin{bmatrix}
%     & - &\hat{\textbf{o}}_1&-\\
%     & &\vdots&\\
%     &-&\hat{\textbf{o}}_{n-i+1}&-
%     \end{bmatrix}
%     \texttt{diag}(\lambda_1,\hdots, \lambda_n)
%     \begin{bmatrix}
%     & | &|&|\\
%     & \hat{\textbf{o}}_1&\hdots&\hat{\textbf{o}}_{n-i+1}\\
%     &|&|&|
%     \end{bmatrix}
%     \right) = \mathcal{N}(\textbf{0},\textbf{C}^{(i)}).
% \end{equation}

% Consequently
% \begin{align}
%     \textbf{T}_{ii} &=  \sqrt{\textbf{Y}^{(i)\top}\textbf{Y}^{(i)}} = \sqrt{\textbf{z}^\top \textbf{C}^{(i)} \textbf{z}}\\
%         &\sim \sqrt{\textbf{z}^\top \texttt{diag}(\lambda(\textbf{C}^{(i)})) \textbf{z}} \\
%         & = \sqrt{\sum_{j=1}^{n-i+1} \lambda(\textbf{C}^{(i)})_{j} \textbf{z}_j^2} \label{eq:tii_chi_squared}
% \end{align}
% where $\textbf{z}\sim\mathcal{N}(\textbf{0}, \textbf{I})$, and $\lambda(\textbf{C}^{(i)})$ are the eigenvalues of $\textbf{C}^{(i)}$.

% Thus {$\textbf{T}_{ii}\sim \sqrt{\sum_{j=i}^n\lambda_j^{(i)}\textbf{z}_j^2 }$} with $\lambda_j^{(i)}$ being the $j$th eigenvalue for $\textbf{C}^{(i)}$.


% \end{proof}

% As a safety check, we now try to retrieve the result in \cite{anderson1962introduction} where it is shown that the Wishart matrices with an identity covariance matrix, $W(\textbf{I},n)$, have a QR decomposition of their matrix factors such that $\textbf{T}_{ii}^2 \sim \chi_{n-i+1}^2$. Thus we apply Proposition \ref{theo:factoriasation} with the identity matrix, i.e. $\textbf{A} = \textbf{I}$.
% \begin{corollary}
% If the eigenvalues of $\textbf{A}$ are identically $1$, then $\textbf{T}_{ii}^2\sim \sum_{j=i}^n\textbf{z}_j^2=\chi_{n-i+1}^2$
% \end{corollary}
% \begin{proof}
% If $\lambda_k=1$ for any $k$, the vector $\textbf{Y}^{(i)}$ defining $\textbf{T}_{ii}$ in \eqref{eq:matr_fact_dist_T} is then distributed as $\textbf{Y}^{(i)}\sim \mathcal{N}(\textbf{0},\textbf{I})$ because of \eqref{eq:matr_fact_dist_Y}. Thus $\lambda_j^{(i)}=1$ for any $j$.
% \end{proof}

% Now that we understand how $\textbf{T}_{ii}$ are drawn, we want to understand how to compute them. To do this, we consider the literature suggesting the Welch-Satterthwaite equation to approximate the summation of $\Gamma$ functions with parameters $\theta_i$ and $k_i$, where $\chi_1^2 \sim \Gamma(1/2,2)$, since it is intractable analytically. This approximation assumes that the summation is a gamma variable with shape parameter $k_{sum}$ and scale parameter $\theta_{sum}$ satisfying
% \begin{align}
%     k_{sum}&=\frac{(\sum_{j=i}^n\theta_jk_j)^2}{\sum_{j=i}^n\theta_j^2k_j}\\
%     \theta_{sum}&=\frac{\sum_{j=1}^n \theta_jk_j}{k_{sum}^i}
% \end{align}
% Thus, since $\lambda\Gamma(k,\theta) = \Gamma(k,\lambda \theta)$, the elements on the diagonal of $\textbf{T}$ are going to be approximate as
% \begin{equation}\label{eq:T_Welch}
%     \textbf{T}_{ii} \sim \sqrt{\alpha^{(i)}\Gamma(\nu^{(i)},2)}
% \end{equation}
% where
% \begin{align}
%     \alpha^{(i)} &=  \frac{\theta_{sum}}{2} = \frac{(\sum_{j=0}^{n-i+1} \lambda_j^{(i)})(\sum_{j=0}^{n-i+1} 2\lambda_j^{(i)}^2)}{2(\sum_{j=0}^{n-i+1} \lambda_j^{(i)})^2}\\
%     & = \frac{\sum_{j=0}^{n-i+1} \lambda_j^{(i)}^2}{\sum_{j=0}^{n-i+1} \lambda_j^{(i)}}\\
%     \nu^{(i)} & = \frac{\left(\sum_{j=0}^{n-i+1} \lambda_j^{(i)}\right)^2}{\sum_{j=0}^{n-i+1} 2\lambda_j^{(i)}^2}
% \end{align}

% As a consequence the determinant of $XAX^\top$ is the product of the elements on the diagonal of the matrix
% \begin{align}
%     |\textbf{XAX}^\top| & = |\textbf{TT}^\top| = |\textbf{T}|^2\\
%     &= \prod_i T_{ii}^2 \sim \prod_i \alpha^{(i)} \prod \Gamma(\nu^{(i)},2)
% \end{align}
% and this allows to use the property that 
% \begin{equation}
%     \mathbb{E}_{\gamma\sim\Gamma(\nu^{(i)},2)}\left[\log\left(\gamma\right)\right] = \log(2) + \varphi(\nu^{(i)})
% \end{equation}
% with $\varphi$ being the digamma function as above.

% Since $\varphi(x) \approx \log(x) - \frac{1}{2x}$,  we assert the following
% \begin{prop}
% Consider a symmetric positive definite matrix $\textbf{A}\in \mathbb{R}^{m\times m}$ and a Gaussian random matrix $\textbf{X} \in \mathbb{R}^{n\times m}$ where the elements are normally distributed. Then the following approximation holds
% \begin{equation}
%     \mathbb{E}_\textbf{X}\left[\log| \textbf{XAX}^\top | \right] \approx \mathbb{E}_\textbf{X}\left[\log\left(\sum_{j=0}^{n-i+1} \lambda_j^{(i)}\right) - \frac{\sum_{j=0}^{n-i+1} \lambda_j^{(i)}^2}{(\sum_{j=0}^{n-i+1} \lambda_j^{(i)})^2} \right]
% \end{equation}
% \end{prop}
% \begin{proof}
% We first have to identify how the different variables of $\textbf{X}$ affect the eigenvalues $\lambda$. As we see in equation \eqref{eq:tii_chi_squared}, the diagonal element $\textbf{T}_{ii}$ depends via $\lambda(\textbf{C}^{(i)})$ to the  columns $(\tilde{\textbf{X}}^\top)_{:,:i-1}$, and via $\textbf{z}$ to the column $(\tilde{\textbf{X}}^\top)_{:,i}$. Consequently we will be able to split the expectation in the following way
% \begin{align}
%     \mathbb{E}_\textbf{X}\left[\log| \textbf{XAX}^\top | \right]& =  \mathbb{E}_\textbf{X}\left[\log\left( \prod_{i=1}^n \textbf{T}_{ii}^2\right) \right] = \sum_{i=1}^n\mathbb{E}_\textbf{X}\left[\log\left( \textbf{T}_{ii}^2\right) \right]\\
%     &= \sum_{i=1}^n\mathbb{E}_\textbf{X}\left[\log\left( \sum_{j=1}^{n-i+1} \lambda(\textbf{C}^{(i)})_j\textbf{z}_j^2\right) \right] \\
%     &= \sum_{i=1}^n\mathbb{E}_{\textbf{X}_{:,:i-1}}\left[\mathbb{E}_{\textbf{X}_{:,i:}}\left[\log\left(  \sum_{j=1}^{n-i+1} \lambda(\textbf{C}^{(i)})_j\textbf{z}_j^2\right) \right]\right]\\
%     & \approx \sum_{i=1}^n\mathbb{E}_{\textbf{X}_{:,:i-1}}\left[\mathbb{E}_{\gamma\sim \Gamma(\nu^{(i)},2)}\left[\log\left(  \alpha^{(i)}\gamma\right) \right]\right]\\
%     & =  \sum_{i=1}^n\mathbb{E}_\textbf{X}\left[ \log( \alpha^{(i)}) + \varphi(\nu^{(i)}) + \log(2) \right]\\
%     & \approx \sum_{i=1}^n\mathbb{E}_\textbf{X}\left[ \log( \alpha^{(i)}) + \log(\nu^{(i)}) - \frac{1}{2\nu^{(i)}} + \log(2) \right]\\
%     & = \sum_{i=1}^n\mathbb{E}_\textbf{X}\left[\log\left( \frac{\sum_{j=0}^{n-i+1} \lambda_j^{(i)}^2}{\sum_{j=0}^{n-i+1} \lambda_j^{(i)}} \frac{\left(\sum_{j=0}^{n-i+1} \lambda_j^{(i)}\right)^2}{\sum_{j=0}^{n-i+1} \lambda_j^{(i)}^2}\right) - \frac{\sum_{j=0}^{n-i+1} \lambda_j^{(i)}^2}{(\sum_{j=0}^{n-i+1} \lambda_j^{(i)})^2}\right] \\
%     & =\sum_{i=1}^n\mathbb{E}_\textbf{X}\left[ \log\left(\sum_{j=0}^{n-i+1} \lambda_j^{(i)}\right) - \frac{\sum_{j=0}^{n-i+1} \lambda_j^{(i)}^2}{(\sum_{j=0}^{n-i+1} \lambda_j^{(i)})^2} \right]
% \end{align}
% \end{proof}

% \subsubsection{Numerical Results}

% In the section above we have introduced different ways to sample the random variable $\textbf{T}_{ii}$. These variables' distribution is determined by the QR decomposition of the random matrix
% \begin{align}\label{eq:QR_dec}
%     &\tilde{\textbf{X}}^\top = 
%     \begin{bmatrix} 
%     &| &| & &|\\
%     &\sqrt{\lambda_1}\textbf{x}_1 &\sqrt{\lambda_2}\textbf{x}_2 & \hdots & \sqrt{\lambda_m}\textbf{x}_{m}\\
%     &| &| & &|
%     \end{bmatrix}^\top = \textbf{O}\textbf{T}.
% \end{align}
% Proposition \ref{theo:factoriasation} asserts that each element $\textbf{T}_{ii}$ is also distributed according to the a quadratic function of normal variables
% \begin{equation}\label{eq:matr_fact_dist_T2}
%     \textbf{T}_{ii}  = \sqrt{\sum_{j=1}^{m-i+1} Y_j^{(i)2}}
% \end{equation}
% where
% \begin{equation}\label{eq:matr_fact_dist_Y2}
%     \textbf{Y}^{(i)}\sim \mathcal{N}\left(\textbf{0},\begin{bmatrix}
%     & - &\hat{\textbf{o}}_1&-\\
%     & &\vdots&\\
%     &-&\hat{\textbf{o}}_{n-i+1}&-
%     \end{bmatrix}
%     \texttt{diag}(\lambda_1,\hdots, \lambda_n)
%     \begin{bmatrix}
%     & | &|&|\\
%     & \hat{\textbf{o}}_1&\hdots&\hat{\textbf{o}}_{n-i+1}\\
%     &|&|&|
%     \end{bmatrix}
%     \right) = \mathcal{N}(\textbf{0},\textbf{C}^{(i)}),
% \end{equation}
% with $\{\hat{\textbf{o}}\}_{j=1}^{m-i+1}$ being a basis of the space complementary to the one defined by the first $i-1$ columns of $\textbf{O}$. Finally we found that the it is possible to approximate \eqref{eq:matr_fact_dist_T2} with the Welch-Satterwaithe equation
% \begin{equation}\label{eq:T_Welch2}
%     \textbf{T}_{ii} \sim \sqrt{\alpha^{(i)}\Gamma(\nu^{(i)},2)}.
% \end{equation}

% To compare how well the distribution of $\textbf{T}_{ii}$ in \eqref{eq:QR_dec}, we will refer to this as (QR), is approximated by the distributions in \eqref{eq:matr_fact_dist_T2} and \eqref{eq:T_Welch2}, respectively ($Y^{(i)}$) and (WS), we will rely on the Kolmogorov-Smirnov test. Given two cumulative distribution functions, the K-S test computes their $L_\infty$ distance and considers the relative p-value, i.e. the probability of obtaining results at least as extreme as the observed results assuming that the null-hypothesis is correct. 

% Since $\textbf{O}$ and $\textbf{T}$ are sequentially generated, the element $\textbf{T}_{ii}$ is dependent on the first $i$ columns of $\tilde{\textbf{X}}^\top$. Thus we will numerically sample the elements $\textbf{T}_{ii}$ by fixing the first $(i-1)$ columns in $\textbf{O}$. Furthermore, we will also sample $\textbf{T}_{ii}$ according to \eqref{eq:matr_fact_dist_T2} considering also the first $(i-1)$ columns of $\textbf{O}$ random. This allows to understand how influential the conditioning on the previous samples is, we will denote these samples with ($Y_r^{(i)}$).


% In Figures \ref{fig:f1}-\ref{fig:f6} we compare the different ways of sampling $\textbf{T}_{ii}$ when $\hat{\textbf{X}}^\top \in \mathbb{R}^{41 \times 40}$ and $\textbf{A}$ is diagonal with elements distributed according to a gamma distribution with shape 1 and scale 10. From Figures \ref{fig:f1}-\ref{fig:f3} we notice how visually the cdf of $\textbf{T}_{ii}$ sampled according to (QR) is approximated accurately by both ($Y^{(i)}$) and (WS), while the distribution according to ($Y_r^{(i)}$) is slightly different for lower elements of the diagonal, i.e. when there are many constraints on the new basis $\{\hat{\textbf{o}}\}_{j=i}^m$. These observations are supported by the KS tests plotted in Figures \ref{fig:f4} and \ref{fig:f5} where the $L_\infty$ distance between the (QR) and respectively the (WS) and the ($Y^{(i)}$) sampling decreases to almost null values when the number of samples increases for any value of $i$, while in the ($Y_r^{(i)}$) case the statistic increases for high values of $i$. Analysing the p-values, we can however notice that when we have many samples, also the hypothesis of (WS) being distributed as (QR) is rejected for almost any $i$, \textbf{this however is suggesting that the approximation is quite accurate as at least 10'000 samples are required to discard this hypothesis?}. Finally, in Figure \ref{fig:f6} all these observations are summarised by plotting the KS statistic and it's relative p-value for different value of $i$ when $10^5$ samples are considered.

% \textbf{Last moment observation: Since we are doing the log determinant, we will consider the elements $\textbf{T}_{ii}$ independently. Thus we should actually consider the distribution not conditioned on the previous columns.}

% \begin{figure}[th!]
%   \begin{minipage}{0.49\textwidth}
%     \includegraphics[width=\textwidth,trim={0.5cm 0.23cm 1.6cm 1.5cm},clip]{Images/Numerics_Factorisation/Hist_cdfs_level0_n_40_m_41_n_samples100000.png}
%     \caption{cdf for $\textbf{T}_{1,1}$}
%     \label{fig:f1}
%   \end{minipage}%
%   \begin{minipage}{0.49\textwidth}
%     \includegraphics[width=\textwidth,trim={0.5cm 0.23cm 1.6cm 1.5cm},clip]{Images/Numerics_Factorisation/Hist_cdfs_level20_n_40_m_41_n_samples100000.png}
%     \caption{cdf for $\textbf{T}_{21,21}$}
%     \label{fig:f2}
%   \end{minipage}\\
%   \centering
%   \begin{minipage}{0.49\textwidth}
%     \includegraphics[width=\textwidth,trim={0.5cm 0.23cm 1.6cm 1.5cm},clip]{Images/Numerics_Factorisation/Hist_cdfs_level36_n_40_m_41_n_samples100000.png}
%     \caption{cdf for $\textbf{T}_{37,37}$}
%     \label{fig:f3}
%   \end{minipage}%
%   \begin{minipage}{0.49\textwidth}
%     \includegraphics[width=\textwidth,trim={0.5cm 0.23cm 1.6cm 1.5cm},clip]{Images/Numerics_Factorisation/Convergence_KS_samples_level_0_n_40_m_41_n_samples100000.png}
%     \caption{Convergence of the KS measure for $\textbf{T}_{1,1}$ when the number of samples increases}
%     \label{fig:f4}
%   \end{minipage}\\
%   \centering
%   \begin{minipage}{0.49\textwidth}
%     \includegraphics[width=\textwidth,trim={0.5cm 0.23cm 1.6cm 1.5cm},clip]{Images/Numerics_Factorisation/Convergence_KS_samples_level_36_n_40_m_41_n_samples100000.png}
%     \caption{Convergence of the KS measure for $\textbf{T}_{37,37}$ when the number of samples increases}
%     \label{fig:f5}
%   \end{minipage}%
%   \begin{minipage}{0.49\textwidth}
%     \includegraphics[width=\textwidth,trim={0.5cm 0.23cm 1.6cm 1.5cm},clip]{Images/Numerics_Factorisation/Convergence_KS_levles_level_n_40_m_41_n_samples100000.png}
%     \caption{KS measure for different $\textbf{T}_{i,i}$ when $10^5$ samples are considered}
%     \label{fig:f6}
%   \end{minipage}
%   \centering
% \end{figure}

% \subsubsection{Approximation of (I1)}

% To apply the previous results to our problem, we have to identify what are the eigenvalues $\lambda_j^{(i)}$. 

% To make the problem treatable we might assume that the matrix 
% \begin{align}
%     \textbf{A} = \begin{bmatrix}
%         &\frac{\sigma_w^2}{n}\mathbb{E}_\textbf{x}[\sigma(\textbf{h}^l)\sigma(\textbf{h}^l)^\top] &\frac{\sqrt{(\sigma_b^2+\sigma_n^2)}\sigma_w}{\sqrt{n}}\mathbb{E}[\sigma(\textbf{h}^l)] \\
%         &\frac{\sqrt{(\sigma_b^2+\sigma_n^2)}\sigma_w}{\sqrt{n}}\mathbb{E}[\sigma(\textbf{h}^l)]^\top &(\sigma_b^2+\sigma_n^2)
%     \end{bmatrix}
% \end{align}
% converges to its expectation on $\mathcal{W}^{:l-1}$. This implies that the different elements of the hidden layer $\textbf{h}_i^{(l)}$ are distributed in the same way, since the rows of $\textbf{W}^{(l)}$ are independent. Thus we have that
% \begin{equation}
%         v^{(l)}  = v_i^{(l)} = \mathbb{E}_\textbf{W,X}[\sigma(\textbf{h}_i)^2].
% \end{equation}
% As a consequence 
% \begin{align}
%     \textbf{A} = \begin{bmatrix}
%         &\frac{\sigma_w^2v^{(l)}}{n}\textbf{I} & \textbf{0}\\
%         & \textbf{0} &(\sigma_b^2+\sigma_n^2)
%     \end{bmatrix}
% \end{align}
% and this implies that the largest eigenvalue is $\hat{\lambda}_{n+1} = \sigma_b^2 + \sigma_n^2$ and the others are all $\hat{\lambda}_j= \sigma_w^2/n*\mathbb{E}_\textbf{X}[\sigma(\textbf{h}_i)]$; we are using a hat symbol over the eigenvalues to distinguish them from the ones defined in the following subsection. For this reason, the first column of $\textbf{O}$ will be almost surely $o_1=\textbf{e}_{n+1}$. Thus at the following iterations the eigenvalues on which we work are all the same since they are defined in the space complementary to the one defined by $\lambda_{n+1}$, i.e.
% \begin{equation}
%     \hat{\lambda}_j^{(i)} = \sigma_w^2 v^{(l)}.
% \end{equation}

% The variable $v^{(l)}$ can be computed numerically following a similar strategy to the one in \cite{Pennington2018}. That is, we iteratively solve the following problem
% \begin{equation}
%     v^{(l)} = \int \sigma\left(  \sqrt{\sigma_w^2 v^{(l-1)} + \sigma_b^2} z \right)^2 \mathcal{D}z.
% \end{equation}

% \subsubsection{Approximation of (I2)}

% To approximate (I2) we can follow a similar techinique to (I1) since
% \begin{align}
%     \bm{\Lambda}_{h^l} &-\frac{1}{\sigma_x^2} \bm{\Sigma}_{xh^l}^\top\bm{\Sigma}_{xh^l} = \mathbb{E}_x[(\textbf{W}^l\sigma(\textbf{h}^l) + \textbf{n}^l + \textbf{b}^l)(\textbf{W}^l\sigma(\textbf{h}^l) + \textbf{n}^l + \textbf{b}^l)^\top]\\
%     & \quad\quad\quad\quad\quad\quad\quad\quad - \frac{1}{\sigma_x^2}\mathbb{E}_x[\textbf{W}^l\sigma(\textbf{h}^l)\textbf{x}^\top]\mathbb{E}_x[\textbf{x}\sigma(\textbf{h}^l)^\top\textbf{W}^l^\top]\\
%     &= \left[\textbf{W}^l, \textbf{b}^l + \textbf{n}^l \right] 
%         \begin{bmatrix}
%             &\mathbb{E}_\textbf{x}[\sigma(\textbf{h}^l)\sigma(\textbf{h}^l)^\top] - \frac{1}{\sigma_x^2}\mathbb{E}_x[\sigma(\textbf{h}^l)\textbf{x}^\top]\mathbb{E}_x[\textbf{x}\sigma(\textbf{h}^l)^\top]& \mathbb{E}_\textbf{x}[\sigma(\textbf{h}^l)] \\
%             & \mathbb{E}_\textbf{x}[\sigma(\textbf{h}^l)]^\top &\textbf{I}
%         \end{bmatrix}
%     \left[\textbf{W}^l, \textbf{b}^l + \textbf{n}^l\right]^\top\\
%     &= \textbf{X}
%     \begin{bmatrix}
%         &\frac{\sigma_w^2}{n}\mathbb{E}_\textbf{x}[\sigma(\textbf{h}^l)\sigma(\textbf{h}^l)^\top] - \frac{1}{\sigma_x^2}\mathbb{E}_x[\sigma(\textbf{h}^l)\textbf{x}^\top]\mathbb{E}_x[\textbf{x}\sigma(\textbf{h}^l)^\top] &\frac{\sqrt{(\sigma_b^2+\sigma_n^2)}\sigma_w}{\sqrt{n}}\mathbb{E}[\sigma(\textbf{h}^l)] \\
%         &\frac{\sqrt{(\sigma_b^2+\sigma_n^2)}\sigma_w}{\sqrt{n}}\mathbb{E}[\sigma(\textbf{h}^l)]^\top &(\sigma_b^2+\sigma_n^2)\textbf{I}
%     \end{bmatrix}\textbf{X}^\top \label{eq:matrix_formulation}\\
%     &= \textbf{XBX}^\top.
% \end{align}

% By using the same approximations for (I1), where $\textbf{B}$ is approximated with its expected value, we get that $\lambda_{n+1} = \sigma_b^2 + \sigma_n^2$ and the others are all $\lambda_j= \sigma_w^2/n(v^{(l)}  -1/\sigma_x^2 c^{(l)})$, where 
% \begin{equation}
%     c^{(l)} = \mathbb{E}_{\mathcal{W}^{(l-1)}} \left[ \sum_{k=1}^n\mathbb{E}_{\textbf{x}}[\sigma(\textbf{h}_i)\textbf{x}_k^\top]\mathbb{E}_{\textbf{x}}[\textbf{x}_k\sigma(\textbf{h}_i)^\top] \right]
% \end{equation}
% For this reason, the first column of $\textbf{O}$ will be $o_1=\textbf{e}_{n+1}$, thus making at the following iterations the eigenvalues on which we work all the same, i.e.
% \begin{equation}
%     \lambda_j^{(i)} = \frac{\sigma_w^2(v^{(l)} - c^{(l)}/\sigma_x^2)}{n}
% \end{equation}

% \subsubsection{Putting all together}

% From what we have defined above, we can then simplify the Mutual information bound via the following equations where $\hat{\lambda}$ defines the eigenvalues relative to (I1) and $\lambda$ the ones of (I2),
% \begin{align}
%     I(\textbf{X},\textbf{h}^l| \mathcal{W}^{:l}) &\geq \frac{1}{2}\mathbb{E}_{\mathcal{W}^{:l}}\left[ \log \left( \left| \bm{\Lambda}_{h^l}\right|  \right)\right]- \mathbb{E}_{\mathcal{W}^{:l}}\left[ \frac{1}{2}\log \left(\left| \bm{\Lambda}_{h^l} -\frac{1}{\sigma_x^2} \bm{\Sigma}_{xh^l}^\top\bm{\Sigma}_{xh^l} \right|  \right)\right]\\
%         & \approx \sum_{i=1}^n \frac{1}{2}\mathbb{E}_{\mathcal{W}^{:l}}\left[ \log\left(\frac{\sum_{j=0}^{n-i+1} \hat{\lambda_j}^{(i)}}{\sum_{j=0}^{n-i+1} \lambda_j^{(i)}}\right) 
%         - \frac{\sum_{j=0}^{n-i+1} \hat{\lambda}_j^{(i)}^2}{(\sum_{j=0}^{n-i+1} \hat{\lambda}_j^{(i)})^2}
%         +  \frac{\sum_{j=0}^{n-i+1} \lambda_j^{(i)}^2}{(\sum_{j=0}^{n-i+1} \lambda_j^{(i)})^2}\right] \\
%         % & \approx \sum_{i=1}^n \frac{1}{2}\mathbb{E}_{\mathcal{W}^{:l}}\left[ \frac{\sum_{j=0}^{n-i+1} \hat{\lambda_j}^{(i)}}{\sum_{j=0}^{n-i+1} \lambda_j^{(i)}} - 1 
%         % - \frac{\sum_{j=0}^{n-i+1} \hat{\lambda}_j^{(i)}^2}{(\sum_{j=0}^{n-i+1} \hat{\lambda}_j^{(i)})^2}
%         % +  \frac{\sum_{j=0}^{n-i+1} \lambda_j^{(i)}^2}{(\sum_{j=0}^{n-i+1} \lambda_j^{(i)})^2}\right]\\
%         & = \frac{1}{2}\mathbb{E}_{\mathcal{W}^{:l}}\left[ \log\left(\frac{\sum_{j=0}^{n} \hat{\lambda_j}}{\sum_{j=0}^{n} \lambda_j}\right) 
%         - \frac{\sum_{j=0}^{n} \hat{\lambda}_j^2}{(\sum_{j=0}^{n} \hat{\lambda}_j^2}
%         +  \frac{\sum_{j=0}^{n} \lambda_j^2}{(\sum_{j=0}^{n} \lambda_j)^2}\right] \\
%         & \quad \quad+ \sum_{i=2}^n \frac{1}{2}\mathbb{E}_{\mathcal{W}^{:l}}\left[ \log\left(\frac{\sum_{j=0}^{n-i+1} \hat{\lambda_j}^{(i)}}{\sum_{j=0}^{n-i+1} \lambda_j^{(i)}}\right) 
%         - \frac{\sum_{j=0}^{n-i+1} \hat{\lambda}_j^{(i)}^2}{(\sum_{j=0}^{n-i+1} \hat{\lambda}_j^{(i)})^2}
%         +  \frac{\sum_{j=0}^{n-i+1} \lambda_j^{(i)}^2}{(\sum_{j=0}^{n-i+1} \lambda_j^{(i)})^2}\right]\\
%         & = \frac{1}{2}\log\left(\frac{ \sigma_w^2v^{(l)} + \sigma_b^2 +\sigma_n^2}{\sigma_w^2(v^{(l)} - c^{(l)}/\sigma_x^2)+ \sigma_b^2 +\sigma_n^2}\right)
%         - \frac{\sigma_w^4v^{(l)2}/n + \sigma_b^4 +\sigma_n^4}{(\sigma_w^2v^{(l)}+ \sigma_b^2 +\sigma_n^2)^2} \\
%         & \quad \quad +  \frac{\sigma_w^4(v^{(l)2} - c^{(l)2}/\sigma_x^4)/n+ \sigma_b^4 +\sigma_n^4}{(\sigma_w^2(v^{(l)} - c^{(l)}/\sigma_x^2)+ \sigma_b^2 +\sigma_n^2)^2} \\
%         & \quad \quad + \sum_{i=2}^n \left[\frac{1}{2}\log\left(\frac{ \sigma_w^2v^{(l)}\frac{n-i+1}{n}}{\sigma_w^2(v^{(l)} - c^{(l)}/\sigma_x^2)\frac{n-i+1}{n}}\right) 
%         - \frac{1}{n-i+1}
%         +  \frac{1}{n-i+1}\right] \\
%         & = \frac{1}{2}\log\left(\frac{ \sigma_w^2v^{(l)} + \sigma_b^2 +\sigma_n^2}{\sigma_w^2(v^{(l)} - c^{(l)}/\sigma_x^2)+ \sigma_b^2 +\sigma_n^2}\left(\frac{ v^{(l)}}{v^{(l)} - c^{(l)}/\sigma_x^2}\right)^{n-1}\right) \\
%         & \quad \quad +  \frac{\sigma_w^4(v^{(l)} - c^{(l)}/\sigma_x^2)^2/n+ \sigma_b^4 +\sigma_n^4}{(\sigma_w^2(v^{(l)} - c^{(l)}/\sigma_x^2)+ \sigma_b^2 +\sigma_n^2)^2} - \frac{\sigma_w^4v^{(l)2}/n + \sigma_b^4 +\sigma_n^4}{(\sigma_w^2v^{(l)}+ \sigma_b^2 +\sigma_n^2)^2}
% \end{align}
% % From the work of \cite{Pennington2018} we could probably approximate $q^l$ independently from the weights $\mathcal{W}$. Furthermore, I have the impression that $c^l$ corresponds to $q^l$ with same $\sigma_w$ but $\sigma_b=0$. If all these hypothesis were to be real, we would then get that
% % \begin{align}
% %     I(\textbf{X},\textbf{h}^l| \mathcal{W}^{:l}) &\geq 
% %         n \log(\frac{q^*}{q^*-c^*})+ \log\left(\frac{\sigma_w^2 + (\sigma_b^2+ \sigma_n^2)/q^*}{\sigma_w^2 + (\sigma_b^2+ \sigma_n^2)/(q^*-c^*)}\right) + \\
% %         & \quad \quad - \frac{\sigma_w^4q^{*2}/n + \sigma_b^4 + \sigma_n^4}{\sigma_w^4q^{*2} + \sigma_b^4 + \sigma_n^4} + \frac{\sigma_w^4(q^{*}-c^*)^2/n + \sigma_b^4 + \sigma_n^4}{\sigma_w^4(q^{*}-c^*)2 + \sigma_b^4 + \sigma_n^4}
% % \end{align}
